# Supplementary material for: Dive into Layers: Neural Network Capacity Bounding using Algebraic Geometry
Source: arXiv:2109.01461 source file (2021-11-04)
Supplement: Supplementary file 1 [file appendix_old.tex]

\section{Appendix}
\renewcommand{\thesubsection}{\Alph{subsection}}
\AtAppendix{\counterwithin{Theorem}{subsection}}
\AtAppendix{\counterwithin{Example}{subsection}}
\AtAppendix{\counterwithin{Property}{subsection}}
\subsection{Algebraic Geometry}
% \begin{definition}[Paffian functions]
% 	Let $U$ be an open domain in $\mathbb{R}^n$, A Pfaffian chain of order $l \geq 1$ and degree $\alpha \geq 1$ in $U$ is a sequence of  real analytic functions  $f_1,f_2,...,f_l$ in $U$ satisfying differential equations 
% 	$$\frac{\partial f_i}{\partial x_j} = P_{i,j}(\mathbf{x}, f_1(\mathbf{x}), ...,f_i(\mathbf{x}))$$
% 	for $i = 1,...,i$ where $P_{i,j} \in \mathbf{R}[x_1,...,x_n,y_1,...,y_i]$ of degree $\leq \alpha$, A function $f$ on $U$ is called Pfaffian function of order $l$ and degree $(\alpha, \beta)$ if 
% 	$$f = P(\mathbf{x},f_1(\mathbf{x}), ...,f_l(\mathbf{x}))$$
% 	where $P \in \mathbf{R}[x_1,...,x_n,y_1,...,y_l]$ us polynomial of degree at most $\beta \geq 1$, the triple $(\alpha, \beta, l)$ are collectively known as the format of the Pfaffian function, and give a useful measure of its complexity. 
% \end{definition}

\begin{definition}[Semi Algebraic Set]
	A semi-algebraic set is a subset $S$ of $\mathbf{R}^n$ for some real closed field $\mathbf{R}$ (for example $\mathbf{R}$ could be the field of real numbers) defined by a finite sequence of polynomial equations (of the form $\mathbf{Q}(x_1,...,x_n)= 0$) and inequalities (of the form $\mathbf{P}(x_1,...,x_n) \geq 0)$, or any finite union of such sets.
\end{definition}

\begin{definition}[Algebraic Set or Variety]
	An algebraic variety $\mathbf{Z}(\mathbf{Q}_i)$ is defined as the set of solutions for a system of polynomial equations $\mathbf{Q}_i$ over the real or complex numbers.
\end{definition}
	As stated above, we can easily know the fact that an algebraic variety is also can be treated as a semi-algebraic set.


\subsection{Simplices and Simplicial Complexes}
\begin{definition}[Simplices]
	The \textit{n-complex}, $\Delta^n$, is the simplest geometric convex hull spanned by a collection of $n + 1$ points in Euclidean space $\mathbb{R}^{n+1}$, generally denoted as $[e_0, e_1, ..., e_n]$, where $e_i = (0,..,0,1,0,..0)$ the i-th position is $1$ and other else is $0$.
\end{definition}

\begin{definition}[Properly Situated]
	An \textit{n-face} of a complex is a subset of the set of vertices of the simplex with order $n +1$, Two simplices are said to be properly situated if their intersection is either empty or a common face of both simplices. 
\end{definition}

\begin{definition}[Simplicial Complexes]
	A simplicial complex $X$ is a finite set of simplices satisfying the following conditions:
	\begin{enumerate}
	    \item For all simplices $\sigma \in X$, $\alpha$ is a face of  $\sigma$ and $\alpha \in X$.
	    \item $\sigma_1, \sigma_2 \in X$ such that $\sigma_1, \sigma_2$ are properly situated.
	\end{enumerate}
\end{definition}
The dimension of a complex is the maximum dimension of the  simplices contained in it.

\begin{definition}[Connected and path-connected]
	A complex $X$ is connected if it can not be represented as the disjoint union of two or more non-empty sub-complexes. A geometric complex is path-connected if there exists a path made of $1$-simplices.
\end{definition}

\subsection{Homology and Co-homology}
Given the set $S$ of vertices of a complex, we define an orientation on the simplex by selecting some particular ordering of $S$, Vertices ordering that differ from this by an odd permutation $\mu$ are then designed as reversed, i.e. $\text{the signature of the permutation} \sign(\mu)$.

Once the orientation is fixed, we can define some concepts.
\begin{definition}[n-chain]
	Given a set of n-simplices $\sigma_1, \sigma_2, ...,\sigma_k$ in a complex and an Abelian group $G$, we define an n-chain  with coefficients in $G$ as a formal sum:
	$$x = \sum_{i} g_i \cdot \sigma_i$$
	where $g_i \in G$.
\end{definition}
Notice that the Abelian group is alternative, such as $\mathbb{Z}, \mathbb{Z}_2$ and $\mathbb{R}$. Without loss of generality we assume that $G= \mathbb{Z}$.

The set of all n-chains equipped with  additive operator forms a new Abelian group, n-chain group denoted as $C_n(X)$.
\begin{definition}[boundary operation]
	Let $\sigma$ be an oriented n-simplex in a complex $X$. The boundary of it is defined as the $(n-1)$-chain of $X$ over $\mathbb{Z}$ given by
	$$\delta_n : C_n(X)\rightarrow C_{n-1}(X)$$
	is a homomorphism from n-chain group to $(n-1)$-chain group.
	$$\delta_n \sigma = \sum_{i=0}^n (-1)^i [v_0,...,v_{i-1}, v_{i+1},...,v_n].$$ 
\end{definition}
Then we can easily verify this matter $\delta_{n+1} \delta_n \sigma = 0$, where $\sigma$ is a $n+1$-simplex. It shows the fact that 
$$C_{n+1}(X) \stackrel{\delta_{n+1}}{\longrightarrow} C_n(X) \stackrel{\delta_{n}}{\longrightarrow}  C_{n-1}(X).$$
i.e. $Img(\delta_{n+1})\subset Ker(\delta_{n}) \subset C_n(X)$.

%\subsection{Singular Homology}
\begin{definition}[singular n-simplex]
	Given a topological space $X$, a singular n-simplex in $X$ is a continuous map $\sigma: \Delta^n \rightarrow X$.
\end{definition}

\begin{definition}
	Let $C_n(X)$ be the  free Abelian group with basis the set of singular n-simplices of $X$. Elements of $C_n(X)$ are called singular n-chains and have finite formal sums:$\sum_{i} g_i\sigma_i$ where $g_i \in \mathbb{Z}$.
\end{definition}

\begin{definition}
	The boundary map $\delta_n : C_n(X)\rightarrow C_{n-1}(X)$ is given by $$\delta_n(\sigma) = \sum_i (-1)^i\sigma|_{[v_0,..,v_{i-1},v_{i+1}, ..., v_n]}$$
	where $\{v_i\}_i$ are the 0-simplices of $\sigma$, that is, the vertices of $\Delta^n$. %v_i : \Delta^0 \rightarrow X$.
\end{definition}
As before, we also can verify that $\delta_{n+1}\delta_n \sigma = 0 $, which suggests that singular homology groups have similar behaviors with the simplicial homology groups.
\begin{definition}
	The singular homology group $H_n(X)$ is defined as the quotient $H_n(X) = Ker(\delta_n) / Img(\delta_{n+1})$.
\end{definition}

\begin{definition}
   Given a chain complex  \[\cdots {\rightarrow} C_{n+1}(X) \stackrel{\delta_{n+1}}{\longrightarrow} C_n(X) \stackrel{\delta_{n}}{\longrightarrow}  C_{n-1}(X)\to\dots\to C_1(X)\stackrel{\delta_{1}}{\longrightarrow}C_0(X)\stackrel{\delta_{0}}{\longrightarrow}0 {\longrightarrow}\cdots\] 
   and a group $G$, we can define the co-chains $C^{*}_n$ to be the respective groups of all  homomorphsims from $C_n$ to $G$:
   $$C^{*}_n = \text{Hom}(C_n, G)$$
    We define the co-boundary map $d_n: C_{n}^{*} \rightarrow C_{n-1}^{*}$ dual to $\delta_n$ as the map sending $\phi \mapsto d_n \phi = \delta^{*}\phi$. For an element $c \in C_n$ and a homomorphism $\phi \in C_{n-1}^{*}$, we have $$d_n \phi(c) = \phi(\delta_n c)$$
    Because $\delta_n\delta_{n+1}=0$, it is easily seen  that $d_{n+1}d_n =0$. In other words, $\text{Img } d_n \subset \text{Ker } d_{n+1}$. With this fact we can define the $n$-th co-homology group as the quotient:
    $$H^n(C; G) =  \text{Ker } d_{n+1} / \text{Img } d_n$$
\end{definition}
\begin{Property}
	If $X_1, ..., X_p$ is the set of all connected components of a complex $X$, and $H_n, H_n^i$ are the homology groups of $X$ and $X_i$ respectively, then $H_n$ is isomorphic to the direct sum $H_n^1\bigoplus \cdots \bigoplus H_n^p$.
\end{Property}
\begin{Property}
	The zero-dimensional homology group of a complex $X$ over $\mathbb{Z}$ is isomorphic to $\mathbb{Z}^p= \bigoplus_p \mathbb{Z}$, where $p$ is  the number of connected components of $X$. 
\end{Property}
%\input{figure/figure1_Betti_number}
The above two properties show topological intuition on the connected components of the dataset. Moreover, the higher-dimensional homology groups show the "higher dimensional holes" of the topological space. From the definition of the homology groups, it is clear that when the dimension of the homology group is no less than the dimension of topological space, it will degenerate to a trivial group i.e., $\{0\}$. 

\begin{example}
a torus, which is defined as cartesian product of two circles $\sT = \mathbb{S}^1 \times \mathbb{S}^1 $, which can be seen as a structure contain $2$ simplices, same as the $n$-dimensional sphere example, $\delta_1 = 0$ so $H_0(\sT) = \sZ$. Now consider $\delta_2$ which maps these two simplices to its boundary, follows that $H_1(\sT) = \sZ\times\sZ$, and $H_2(\sT) = \Ker\delta_2$ since there are no $3$ simplices, hence $H_2(\sT)=  \sZ$.
\end{example}

\begin{definition}[Reduced homology groups]
   the augmented chain complex is defined as \[\cdots {\rightarrow} C_{n+1}(X) \stackrel{\delta_{n+1}}{\longrightarrow} C_n(X) \stackrel{\delta_{n}}{\longrightarrow}  C_{n-1}(X)\to\dots\to C_1(X)\stackrel{\delta_{1}}{\longrightarrow}C_0(X)\stackrel{\epsilon}{\longrightarrow}\sZ\stackrel{\delta_{0}}{\longrightarrow}0 {\rightarrow}\cdots\]
where $\epsilon(\sum_i n_i\sigma_i) = \sum_i n_i$, then
the reduced homology groups $\widetilde{H}_i(X) = \Ker(\delta_i)/\Img(\delta_{i+1})$ for $i>0$, and $\Widetilde{H}_0(X) = \ker(\epsilon)/\Img(\delta_1)$. One can show that $H_i(X) = \widetilde{H}_i(X)$ for $i>0$ and $H_0(X) = \widetilde{H}_0(X) \bigoplus \sZ$.
\end{definition}



% 	\begin{definition}[cycle group and boundary group]
% 		We call the kernel of boundary homomorphism $\delta_n: C_n(K)\rightarrow C_{n-1}(K)$ of a topological space $K$ the close cycle group denoted as $Z_n(K)$, which is the normal subgroup of $C_n(K)$,
% 		the element in the close cycle group is said as a cycle, and the image of $\delta_{n+1}: C_{n+ 1}(K)\rightarrow C_{n}(K)$ is the boundary group denoted as $B_n(K)$, the element in this group is called a boundary chain.
% 	\end{definition}
% 	As mentioned above, An quotient group  $Z_n(K)/B_n(K)$can be generated, denoted as $H_n(K)$, which is the so-called homology group. 
% 	\begin{definition}[Homology group]
% 		We call the quotient group $H_n(K)= Z_n(K)/B_n(K)$ homology group.
% 	\end{definition}
% 	\begin{definition}[Betti number]
% 		The rank of $H_n(K)$ is called n-dimensional Betti number $b_n$
% 	\end{definition}

To study the relations of the Betti numbers of sets with those of their intersections and unions, we use Mayer-Vietoris sequence, first we introduce the concept of exact sequence.
\input{content/proofs/Def_exact_sequence}
\input{content/proofs/Def_double_complex}
\subsection{Proof of Lemma~\ref{lemma:complex_isomorphism}}
\input{content/proofs/Lemma_complex_isomorphism}
\subsection{Proof of Lemma~\ref{lemma:complex_exact}}
\input{content/proofs/Lemma_complex_exact}
\subsection{Related Theorems}
\begin{theorem}[\cite{Basu2001}]
	Let $\mathbf{R}$ be a real closed field and let $S \subset \mathbf{R}^k$ be the set define by the conjunction of $n$ inequalities.
	$$\mathbf{P}_1 \geq 0, \cdots, \mathbf{P}_n \geq 0$$
	$\mathbf{P}\in \mathbf{R}[X_1,...,X_k], deg(\mathbf{P}_i) \leq d, 1\leq i\leq n$, contained in a variety $\mathbf{Z(Q)}$ of real dimension $k'$ with $deg(\mathbf{Q}) \leq d$. Then we have
	$$b_i(S) \leq \sum_{j=0}^{k'-i} \binom{n}{j} 2^{j+1} d(2d - 1)^{k- 1} \leq \binom{n}{k'-i} \mathbf{O}(d^k).$$	
\end{theorem}
and its dual result:
\begin{theorem}[\cite{Basu2001}]
	Let $\mathbf{R}$ be a real closed field and let $S \subset \mathbf{R}^k$ be the set define by the disjunction of $n$ inequalities.
	$$\mathbf{P}_1 \geq 0, \cdots, \mathbf{P}_n \geq 0$$
	$\mathbf{P}\in \mathbf{R}[X_1,...,X_k], deg(\mathbf{P}_i) \leq d, 1\leq i\leq n$. Then we have
	$$b_i(S) \leq \sum_{j=0}^{i+1} \binom{n}{j} 3^{j} d(2d - 1)^{k- 1} \leq \binom{n}{i+1} \mathbf{O}(d^k).$$	
\end{theorem}
